# Supplementary material for: Accelerated Prediction of Temperature-Dependent Lattice Thermal Conductivity via Ensembled Machine Learning Models
Source: arXiv:2511.13202 source file (2025-11-21)
Supplement: Supplementary file 2 [file supplementary_file.pdf]

**Supplementary Information for “Accelerated Prediction of  
Temperature-Dependent Lattice Thermal Conductivity via Ensembled  
Machine Learning Models”**

Piyush Paliwal<sup>1</sup> and Aftab Alam<sup>1,2\*</sup>

<sup>1</sup>*Center for Machine Intelligence and Data Science (CMInDS),  
Indian Institute of Technology Bombay, Powai, Mumbai 400076, India and*

<sup>2</sup>*Department of Physics, Indian Institute of  
Technology Bombay, Powai, Mumbai 400076, India*

Here, we provide further auxiliary details regarding those compounds used for training, compositional and structural features, feature importances, and formulation of all the models.

---

\* [aftab@iitb.ac.in](mailto:aftab@iitb.ac.in)

# I. COMPOUND DATA FOR MODEL TRAINING

TABLE S1. Data for 116 Compounds with their corresponding Space Group[1].

| Sr. No. | Compound Name | Space Group  | Sr. No. | Compound Name      | Space Group  |
|---------|---------------|--------------|---------|--------------------|--------------|
| 1       | AlAs          | $F\bar{4}3m$ | 59      | HfSe <sub>2</sub>  | $P\bar{3}m1$ |
| 2       | AlP           | $F\bar{4}3m$ | 60      | HfSnPd             | $F\bar{4}3m$ |
| 3       | AlSb          | $F\bar{4}3m$ | 61      | HoHSe              | $P\bar{6}m2$ |
| 4       | BP            | $F\bar{4}3m$ | 62      | HoNiSb             | $F\bar{4}3m$ |
| 5       | BSb           | $F\bar{4}3m$ | 63      | HoSbPd             | $F\bar{4}3m$ |
| 6       | BaS           | $F\bar{4}3m$ | 64      | HoSbPt             | $F\bar{4}3m$ |
| 7       | BaSe          | $Fm\bar{3}m$ | 65      | HoSnAu             | $F\bar{4}3m$ |
| 8       | BaTe          | $Fm\bar{3}m$ | 66      | K <sub>2</sub> S   | $Fm\bar{3}m$ |
| 9       | BeS           | $F\bar{4}3m$ | 67      | K <sub>2</sub> Se  | $Fm\bar{3}m$ |
| 10      | BeSe          | $F\bar{4}3m$ | 68      | K <sub>2</sub> Te  | $Fm\bar{3}m$ |
| 11      | BeTe          | $F\bar{4}3m$ | 69      | LaCoTe             | $F\bar{4}3m$ |
| 12      | BiB           | $F\bar{4}3m$ | 70      | Li <sub>2</sub> S  | $Fm\bar{3}m$ |
| 13      | CaS           | $Fm\bar{3}m$ | 71      | Li <sub>2</sub> Se | $Fm\bar{3}m$ |
| 14      | CaSe          | $F\bar{4}3m$ | 72      | Li <sub>2</sub> Te | $Fm\bar{3}m$ |
| 15      | CaSe          | $Fm\bar{3}m$ | 73      | LiFeP              | $I4mm$       |
| 16      | CaTe          | $Fm\bar{3}m$ | 74      | LiGaSi             | $F\bar{4}3m$ |
| 17      | CdS           | $F\bar{4}3m$ | 75      | LiMgP              | $F\bar{4}3m$ |
| 18      | CdSe          | $F\bar{4}3m$ | 76      | LuSbPt             | $F\bar{4}3m$ |
| 19      | CdTe          | $F\bar{4}3m$ | 77      | MoS <sub>2</sub>   | $P\bar{6}m2$ |
| 20      | GaAs          | $F\bar{4}3m$ | 78      | MoSe <sub>2</sub>  | $P\bar{6}m2$ |
| 21      | GaP           | $F\bar{4}3m$ | 79      | MoSe <sub>2</sub>  | $R\bar{3}m$  |
| 22      | GeC           | $F\bar{4}3m$ | 80      | Na <sub>2</sub> S  | $Fm\bar{3}m$ |
| 23      | InP           | $F\bar{4}3m$ | 81      | Na <sub>2</sub> Se | $Fm\bar{3}m$ |
| 24      | MgS           | $F\bar{4}3m$ | 82      | Na <sub>2</sub> Te | $Fm\bar{3}m$ |
| 25      | MgS           | $Fm\bar{3}m$ | 83      | NbCoSn             | $F\bar{4}3m$ |

| Sr. No. | Compound<br>Name   | Space<br>Group | Sr. No. | Compound<br>Name     | Space<br>Group |
|---------|--------------------|----------------|---------|----------------------|----------------|
| 26      | MgSe               | $F\bar{4}3m$   | 84      | NbFeSb               | $F\bar{4}3m$   |
| 27      | MgTe               | $Fm\bar{3}m$   | 85      | NbSbRu               | $F\bar{4}3m$   |
| 28      | MgTe               | $F\bar{4}3m$   | 86      | PbF <sub>2</sub>     | $Fm\bar{3}m$   |
| 29      | PbS                | $Fm\bar{3}m$   | 87      | PbI <sub>2</sub>     | $R\bar{3}m$    |
| 30      | PbSe               | $Fm\bar{3}m$   | 88      | PbI <sub>2</sub>     | $P\bar{3}m1$   |
| 31      | SiC                | $F\bar{4}3m$   | 89      | PtS <sub>2</sub>     | $P\bar{3}m1$   |
| 32      | SiSn               | $F\bar{4}3m$   | 90      | Rb <sub>2</sub> S    | $Fm\bar{3}m$   |
| 33      | SnC                | $F\bar{4}3m$   | 91      | Rb <sub>2</sub> Se   | $Fm\bar{3}m$   |
| 34      | SnS                | $Fm\bar{3}m$   | 92      | Rb <sub>2</sub> Te   | $Fm\bar{3}m$   |
| 35      | SnSe               | $Fm\bar{3}m$   | 93      | ScCoTe               | $F\bar{4}3m$   |
| 36      | SrTe               | $Fm\bar{3}m$   | 94      | ScSnAu               | $F\bar{4}3m$   |
| 37      | TePb               | $Fm\bar{3}m$   | 95      | SmSnAu               | $F\bar{4}3m$   |
| 38      | TlBr               | $Pm\bar{3}m$   | 96      | SnO <sub>2</sub>     | $R\bar{3}m$    |
| 39      | TlBr               | $Fm\bar{3}m$   | 97      | SeTePd               | $F\bar{4}3m$   |
| 40      | TlCl               | $Pm\bar{3}m$   | 98      | TaTlPt               | $F\bar{4}3m$   |
| 41      | TlCl               | $Fm\bar{3}m$   | 99      | Te <sub>2</sub> Mo   | $P\bar{6}m2$   |
| 42      | TlI                | $Pm\bar{3}m$   | 100     | AlP                  | $P6_3mc$       |
| 43      | BaLiP              | $P\bar{6}m2$   | 101     | B <sub>2</sub> AsP   | $P\bar{4}m2$   |
| 44      | BiTeI              | $P3m1$         | 102     | BP                   | $P6_3mc$       |
| 45      | Ca <sub>2</sub> Ge | $Fm\bar{3}m$   | 103     | Ba <sub>2</sub> AgSb | $Fm\bar{3}m$   |
| 46      | Ca <sub>2</sub> Pb | $Fm\bar{3}m$   | 104     | Ba <sub>2</sub> BiAu | $Fm\bar{3}m$   |
| 47      | Ca <sub>2</sub> Si | $Fm\bar{3}m$   | 105     | Ba <sub>2</sub> PCl  | $R\bar{3}m$    |
| 48      | Ca <sub>2</sub> Sn | $Fm\bar{3}m$   | 106     | Ba <sub>2</sub> SbAu | $Fm\bar{3}m$   |
| 49      | CeSe <sub>2</sub>  | $Fm\bar{3}m$   | 107     | CdS                  | $P6_3mc$       |
| 50      | Cs <sub>2</sub> Se | $Fm\bar{3}m$   | 108     | CdSe                 | $P6_3mc$       |
| 51      | DySbPt             | $F\bar{4}3m$   | 109     | CdTe                 | $P6_3mc$       |

| Sr. No. | Compound<br>Name | Space<br>Group | Sr. No. | Compound<br>Name    | Space<br>Group |
|---------|------------------|----------------|---------|---------------------|----------------|
| 52      | ErNiSb           | $F\bar{4}3m$   | 110     | CsHoS <sub>2</sub>  | $R\bar{3}m$    |
| 53      | ErSbPd           | $F\bar{4}3m$   | 111     | CsK <sub>2</sub> Sb | $Fm\bar{3}m$   |
| 54      | ErSbPt           | $F\bar{4}3m$   | 112     | DyTlS <sub>2</sub>  | $R\bar{3}m$    |
| 55      | ErSnAu           | $F\bar{4}3m$   | 113     | DyTlSe <sub>2</sub> | $R\bar{3}m$    |
| 56      | FeS <sub>2</sub> | $R\bar{3}m$    | 114     | DyTlTe <sub>2</sub> | $R\bar{3}m$    |
| 57      | HfNiSn           | $F\bar{4}3m$   | 115     | GaAs                | $P6_3mc$       |
| 58      | HfS <sub>2</sub> | $P\bar{3}m1$   | 116     | GaP                 | $P6_3mc$       |

TABLE S2. Data for the rest of the compounds (117 to 150) in the training data-set and their corresponding Space Group.

| Sr. No. | Compound<br>Name                  | Space Group  | Ref. |
|---------|-----------------------------------|--------------|------|
| 117     | Ag <sub>2</sub> GeTe <sub>3</sub> | $Cmc2_1$     | [2]  |
| 118     | Ag <sub>2</sub> GeS <sub>3</sub>  | $Cmc2_1$     | [2]  |
| 119     | Ag <sub>2</sub> GeSe <sub>3</sub> | $Cmc2_1$     | [2]  |
| 120     | BeSiSb <sub>2</sub>               | $I\bar{4}2d$ | [3]  |
| 121     | BiSeI                             | $Pnma$       | [4]  |
| 122     | CoNiFe                            | $F\bar{4}3m$ | [5]  |
| 123     | CsZnSb                            | $P6_3/mmc$   | [6]  |
| 124     | Li <sub>2</sub> CaPb              | $Fm\bar{3}m$ | [7]  |
| 125     | RbZnSb                            | $P6_3/mmc$   | [6]  |
| 126     | MgSiSb <sub>2</sub>               | $I\bar{4}2d$ | [3]  |
| 127     | Na <sub>2</sub> MgSn              | $P6_3/mmc$   | [8]  |
| 128     | Na <sub>2</sub> MgPb              | $P6_3/mmc$   | [8]  |
| 129     | CaP <sub>3</sub>                  | $P\bar{1}$   | [9]  |
| 130     | NiHfSn                            | $F\bar{4}3m$ | [10] |
| 131     | NiTiSn                            | $F\bar{4}3m$ | [10] |
| 132     | RhBiHf                            | $F\bar{4}3m$ | [11] |
| 133     | RhBiTi                            | $F\bar{4}3m$ | [11] |
| 134     | Sr <sub>2</sub> Ge                | $Pnma$       | [12] |
| 135     | ScCuTe <sub>2</sub>               | $P3m1$       | [13] |
| 136     | ScCuSe <sub>2</sub>               | $P3m1$       | [13] |
| 137     | ScCuS <sub>2</sub>                | $P3m1$       | [13] |
| 138     | Tl <sub>3</sub> VSe <sub>4</sub>  | $I\bar{4}3m$ | [14] |
| 139     | Cu <sub>3</sub> VSe <sub>4</sub>  | $P\bar{4}3m$ | [14] |
| 140     | CuBiTeO                           | $P4/nmm$     | [15] |
| 141     | ZrCoSb                            | $F\bar{4}3m$ | [16] |

| Sr. No. | Compound Name      | Space Group  | Ref. |
|---------|--------------------|--------------|------|
| 142     | HfCoSb             | $F\bar{4}3m$ | [16] |
| 143     | LiMgN              | $F\bar{4}3m$ | [17] |
| 144     | LiZnN              | $F\bar{4}3m$ | [17] |
| 145     | ScRhTe             | $F\bar{4}3m$ | [18] |
| 146     | LiScPtGe           | $F\bar{4}3m$ | [19] |
| 147     | LiYPtSn            | $F\bar{4}3m$ | [19] |
| 148     | LiYPdPb            | $F\bar{4}3m$ | [19] |
| 149     | BaAgP              | $P6_3/mmc$   | [20] |
| 150     | Sr <sub>2</sub> Si | $Pnma$       | [12] |

**Target Property: Lattice Thermal Conductivity ( $\kappa_L$ ):** The lattice thermal conductivity ( $\kappa_L$ ) values (between 100K to 1200K) for all 150 compounds listed in Table S1 and Table S2 were obtained from density functional theory (DFT) calculations performed at the Perdew–Burke–Ernzerhof (PBE) level of the generalized gradient approximation (GGA). The phonon properties were computed by explicitly considering third-order interatomic force constants (IFCs), and the lattice thermal conductivities were subsequently evaluated by solving the phonon Boltzmann transport equation (BTE). These  $\kappa_L$  values were used as the reference dataset for training and validating the machine learning models presented in this study.

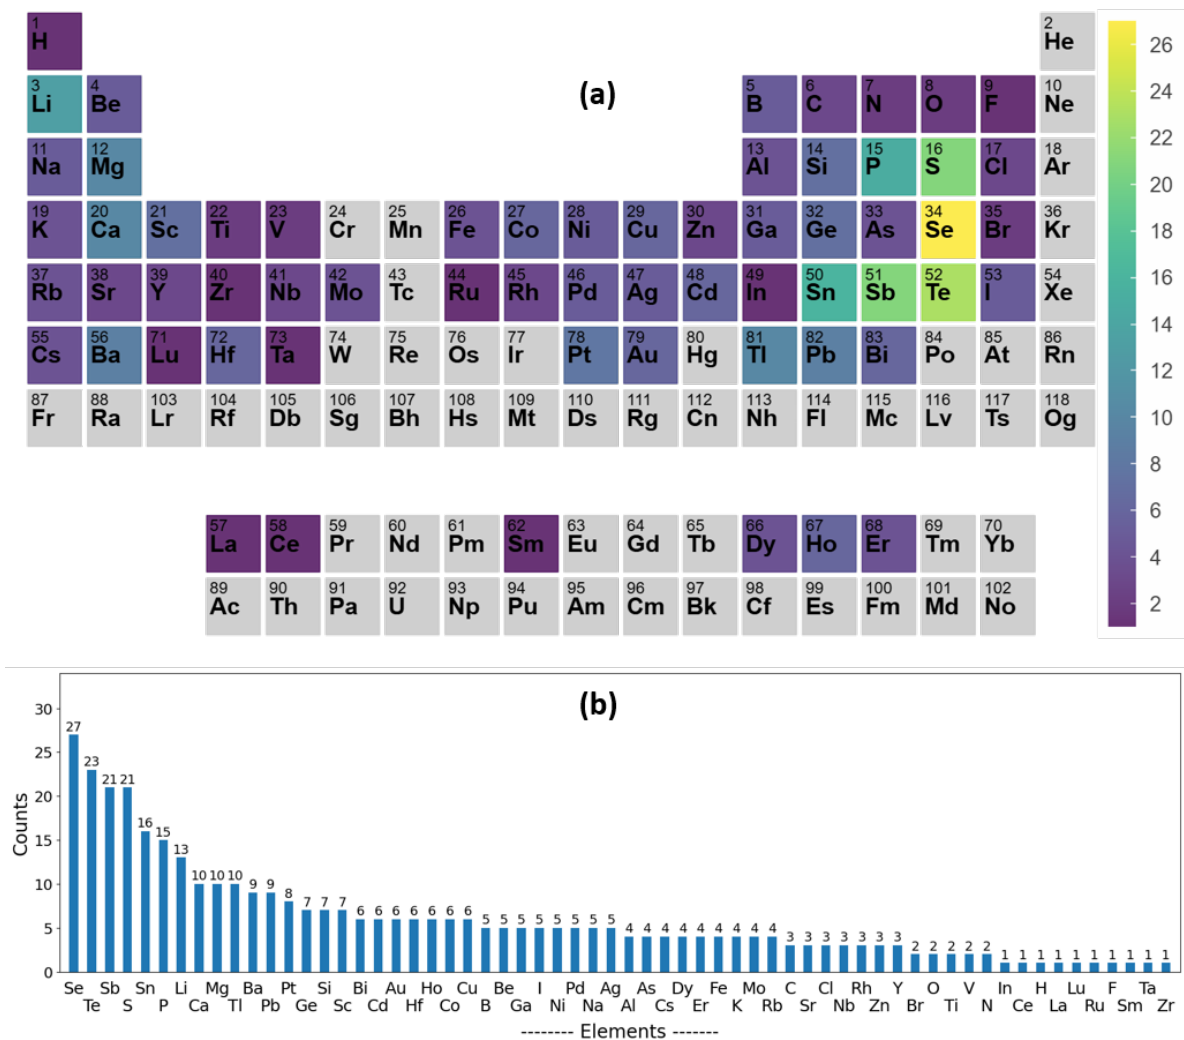

FIG. S1. The distribution of elements across the dataset of 150 compounds in (a) a periodic table map (color bar indicates the frequency of occurrence of each element) (b) a histogram representing a complementary quantitative overview.



TABLE S3. 22 Elemental properties used to generate the composition features.

| Elemental property                 | Elemental property      |
|------------------------------------|-------------------------|
| Atomic number                      | s valance electrons     |
| Atomic weight                      | p valance electrons     |
| Electronegativity                  | d valance electrons     |
| Bandgap of ground state            | f valance electrons     |
| Space group number of ground state | Total valance electrons |
| Mendeleeev number                  | Unfilled s states       |
| Column                             | Unfilled p states       |
| Row                                | Unfilled d states       |
| Column radius                      | Unfilled f states       |
| Specific volume of ground state    | Total unfilled states   |
| Magnetic moment of ground state    | Melting temperature     |

## II. COMPOSITIONAL AND STRUCTURE FEATURES

The features used in this work were obtained from the Material Agonistic Platform for Informatics and Exploration (Magpie)[21]. In broad category, feature space is divided mainly into two categories: Structural characteristics (126 in number) and composition characteristics (145 in number). This results in a total of 271 features corresponding to each crystal structure. Both kinds of features are generated from VASP formatted structure file (namely POSCAR) of the concerned compound. A brief description of each feature category is provided below. For detailed information, refer to the paper by Ward et al. and its Supplementary Section[22].

### A. Composition Features

Table S3 display the elemental properties used to generate compositional features. Table S4 provides 145 composition features generated using 6 equations of mean, mean absolute deviation, range, maximum, minimum and mode fraction of each element in the crystal collectively with its 22 properties as provided in Table S3.

TABLE S4. Complete list of Composition features.

| Sr. No. | Feature Name            | Sr. No. | Feature Name       |
|---------|-------------------------|---------|--------------------|
| 1       | NComp                   | 74      | maxdiff_NfValence  |
| 2       | Comp_L2Norm             | 75      | dev_NfValence      |
| 3       | Comp_L3Norm             | 76      | max_NfValence      |
| 4       | Comp_L5Norm             | 77      | min_NfValence      |
| 5       | Comp_L7Norm             | 78      | most_NfValence     |
| 6       | Comp_L10Norm            | 79      | mean_NValance      |
| 7       | mean_Number             | 80      | maxdiff_NValance   |
| 8       | maxdiff_Number          | 81      | dev_NValance       |
| 9       | dev_Number              | 82      | max_NValance       |
| 10      | max_Number              | 83      | min_NValance       |
| 11      | min_Number              | 84      | most_NValance      |
| 12      | most_Number             | 85      | mean_NsUnfilled    |
| 13      | mean_MendeleevNumber    | 86      | maxdiff_NsUnfilled |
| 14      | maxdiff_MendeleevNumber | 87      | dev_NsUnfilled     |
| 15      | dev_MendeleevNumber     | 88      | max_NsUnfilled     |
| 16      | max_MendeleevNumber     | 89      | min_NsUnfilled     |
| 17      | min_MendeleevNumber     | 90      | most_NsUnfilled    |
| 18      | most_MendeleevNumber    | 91      | mean_NpUnfilled    |
| 19      | mean_AtomicWeight       | 92      | maxdiff_NpUnfilled |
| 20      | maxdiff_AtomicWeight    | 93      | dev_NpUnfilled     |
| 21      | dev_AtomicWeight        | 94      | max_NpUnfilled     |
| 22      | max_AtomicWeight        | 95      | min_NpUnfilled     |
| 23      | min_AtomicWeight        | 96      | most_NpUnfilled    |
| 24      | most_AtomicWeight       | 97      | mean_NdUnfilled    |
| 25      | mean_MeltingT           | 98      | maxdiff_NdUnfilled |
| 26      | maxdiff_MeltingT        | 99      | dev_NdUnfilled     |
| 27      | dev_MeltingT            | 100     | max_NdUnfilled     |

| Sr. No. | Feature Name              | Sr. No. | Feature Name        |
|---------|---------------------------|---------|---------------------|
| 28      | max_MeltingT              | 101     | min_NdUnfilled      |
| 29      | min_MeltingT              | 102     | most_NdUnfilled     |
| 30      | most_MeltingT             | 103     | mean_NfUnfilled     |
| 31      | mean_Column               | 104     | maxdiff_NfUnfilled  |
| 32      | maxdiff_Column            | 105     | dev_NfUnfilled      |
| 33      | dev_Column                | 106     | max_NfUnfilled      |
| 34      | max_Column                | 107     | min_NfUnfilled      |
| 35      | min_Column                | 108     | most_NfUnfilled     |
| 36      | most_Column               | 109     | mean_NUnfilled      |
| 37      | mean_Row                  | 110     | maxdiff_NUnfilled   |
| 38      | maxdiff_Row               | 111     | dev_NUnfilled       |
| 39      | dev_Row                   | 112     | max_NUnfilled       |
| 40      | max_Row                   | 113     | min_NUnfilled       |
| 41      | min_Row                   | 114     | most_NUnfilled      |
| 42      | most_Row                  | 115     | mean_GSvolume_pa    |
| 43      | mean_CovalentRadius       | 116     | maxdiff_GSvolume_pa |
| 44      | maxdiff_CovalentRadius    | 117     | dev_GSvolume_pa     |
| 45      | dev_CovalentRadius        | 118     | max_GSvolume_pa     |
| 46      | max_CovalentRadius        | 119     | min_GSvolume_pa     |
| 47      | min_CovalentRadius        | 120     | most_GSvolume_pa    |
| 48      | most_CovalentRadius       | 121     | mean_GSbandgap      |
| 49      | mean_Electronegativity    | 122     | maxdiff_GSbandgap   |
| 50      | maxdiff_Electronegativity | 123     | dev_GSbandgap       |
| 51      | dev_Electronegativity     | 124     | max_GSbandgap       |
| 52      | max_Electronegativity     | 125     | min_GSbandgap       |
| 53      | min_Electronegativity     | 126     | most_GSbandgap      |
| 54      | most_Electronegativity    | 127     | mean_GSmagmom       |
| 55      | mean_NsValence            | 128     | maxdiff_GSmagmom    |

| Sr. No. | Feature Name      | Sr. No. | Feature Name             |
|---------|-------------------|---------|--------------------------|
| 56      | maxdiff_NsValence | 129     | dev_GSmagmom             |
| 57      | dev_NsValence     | 130     | max_GSmagmom             |
| 58      | max_NsValence     | 131     | min_GSmagmom             |
| 59      | min_NsValence     | 132     | most_GSmagmom            |
| 60      | most_NsValence    | 133     | mean_SpaceGroupNumber    |
| 61      | mean_NpValence    | 134     | maxdiff_SpaceGroupNumber |
| 62      | maxdiff_NpValence | 135     | dev_SpaceGroupNumber     |
| 63      | dev_NpValence     | 136     | max_SpaceGroupNumber     |
| 64      | max_NpValence     | 137     | min_SpaceGroupNumber     |
| 65      | min_NpValence     | 138     | most_SpaceGroupNumber    |
| 66      | most_NpValence    | 139     | frac_sValence            |
| 67      | mean_NdValence    | 140     | frac_pValence            |
| 68      | maxdiff_NdValence | 141     | frac_dValence            |
| 69      | dev_NdValence     | 142     | frac_fValence            |
| 70      | max_NdValence     | 143     | CanFormIonic             |
| 71      | min_NdValence     | 144     | MaxIonicChar             |
| 72      | most_NdValence    | 145     | MeanIonicChar            |
| 73      | mean_NfValence    |         |                          |

## B. Structural Features

Table S5 provides 126 structural features. These features are generated using mean, maximum, variance, and range of various structural properties.

TABLE S5. Complete list of structural features.

| Sr. No. | Feature Name                            | Sr. No. | Feature Name                             |
|---------|-----------------------------------------|---------|------------------------------------------|
| 1       | max_NeighDiff_shell1_GSvolume_pa        | 64      | mean_NeighDiff_shell1_NfUnfilled         |
| 2       | mean_WCMagnitude_Shell2                 | 65      | min_NeighDiff_shell1_MeltingT            |
| 3       | mean_WCMagnitude_Shell1                 | 66      | max_NeighDiff_shell1_NValance            |
| 4       | mean_NeighDiff_shell1_Row               | 67      | min_NeighDiff_shell1_CovalentRadius      |
| 5       | var_BondLengthVariation                 | 68      | range_NeighDiff_shell1_Electronegativity |
| 6       | var_NeighDiff_shell1_SpaceGroupNumber   | 69      | var_EffectiveCoordination                |
| 7       | range_NeighDiff_shell1_SpaceGroupNumber | 70      | range_NeighDiff_shell1_NsUnfilled        |
| 8       | range_NeighDiff_shell1_AtomicWeight     | 71      | max_NeighDiff_shell1_NsValence           |
| 9       | max_NeighDiff_shell1_Column             | 72      | min_NeighDiff_shell1_NUnfilled           |
| 10      | max_NeighDiff_shell1_GSmagmom           | 73      | min_NeighDiff_shell1_NpValence           |
| 11      | min_NeighDiff_shell1_NfUnfilled         | 74      | var_NeighDiff_shell1_NfUnfilled          |
| 12      | mean_NeighDiff_shell1_AtomicWeight      | 75      | mean_WCMagnitude_Shell3                  |
| 13      | max_NeighDiff_shell1_MendeleevNumber    | 76      | mean_NeighDiff_shell1_NfValence          |
| 14      | range_NeighDiff_shell1_Row              | 77      | mean_NeighDiff_shell1_NdUnfilled         |
| 15      | range_NeighDiff_shell1_NpValence        | 78      | mean_NeighDiff_shell1_SpaceGroupNumber   |
| 16      | min_NeighDiff_shell1_SpaceGroupNumber   | 79      | max_NeighDiff_shell1_NdUnfilled          |
| 17      | var_NeighDiff_shell1_GSbandgap          | 80      | max_NeighDiff_shell1_GSbandgap           |
| 18      | min_NeighDiff_shell1_NValance           | 81      | max_NeighDiff_shell1_SpaceGroupNumber    |
| 19      | mean_NeighDiff_shell1_GSbandgap         | 82      | var_NeighDiff_shell1_Number              |
| 20      | max_MeanBondLength                      | 83      | min_NeighDiff_shell1_NpUnfilled          |
| 21      | max_NeighDiff_shell1_Row                | 84      | max_BondLengthVariation                  |
| 22      | range_NeighDiff_shell1_NfValence        | 85      | max_NeighDiff_shell1_NUnfilled           |
| 23      | min_NeighDiff_shell1_GSvolume_pa        | 86      | max_NeighDiff_shell1_AtomicWeight        |
| 24      | range_NeighDiff_shell1_NValance         | 87      | min_NeighDiff_shell1_NfValence           |
| 25      | min_MeanBondLength                      | 88      | var_NeighDiff_shell1_MeltingT            |
| 26      | mean_NeighDiff_shell1_Number            | 89      | mean_NeighDiff_shell1_MendeleevNumber    |
| 27      | min_BondLengthVariation                 | 90      | var_NeighDiff_shell1_AtomicWeight        |

| Sr. No. | Feature Name                           | Sr. No. | Feature Name                            |
|---------|----------------------------------------|---------|-----------------------------------------|
| 28      | mean_NeighDiff_shell1_CovalentRadius   | 91      | min_NeighDiff_shell1_MendeleevNumber    |
| 29      | var_NeighDiff_shell1_GSmagmom          | 92      | min_NeighDiff_shell1_NsUnfilled         |
| 30      | range_NeighDiff_shell1_GSbandgap       | 93      | var_NeighDiff_shell1_CovalentRadius     |
| 31      | mean_NeighDiff_shell1_NpUnfilled       | 94      | var_NeighDiff_shell1_NValance           |
| 32      | range_NeighDiff_shell1_NfUnfilled      | 95      | var_NeighDiff_shell1_Column             |
| 33      | max_NeighDiff_shell1_NpValence         | 96      | var_NeighDiff_shell1_NdUnfilled         |
| 34      | mean_NeighDiff_shell1_NdValence        | 97      | min_NeighDiff_shell1_GSmagmom           |
| 35      | mean_NeighDiff_shell1_NsValence        | 98      | min_NeighDiff_shell1_GSbandgap          |
| 36      | range_NeighDiff_shell1_Number          | 99      | MaxPackingEfficiency                    |
| 37      | range_NeighDiff_shell1_CovalentRadius  | 100     | range_NeighDiff_shell1_MeltingT         |
| 38      | mean_NeighDiff_shell1_GSvolume_pa      | 101     | mean_NeighDiff_shell1_Electronegativity |
| 39      | var_NeighDiff_shell1_NsValence         | 102     | min_EffectiveCoordination               |
| 40      | max_NeighDiff_shell1_Number            | 103     | mean_NeighDiff_shell1_NsUnfilled        |
| 41      | min_NeighDiff_shell1_Number            | 104     | range_NeighDiff_shell1_NsValence        |
| 42      | var_NeighDiff_shell1_NsUnfilled        | 105     | min_NeighDiff_shell1_NdUnfilled         |
| 43      | var_NeighDiff_shell1_NfValence         | 106     | var_NeighDiff_shell1_Row                |
| 44      | max_NeighDiff_shell1_MeltingT          | 107     | min_NeighDiff_shell1_NsValence          |
| 45      | var_NeighDiff_shell1_NdValence         | 108     | min_NeighDiff_shell1_Row                |
| 46      | min_NeighDiff_shell1_NdValence         | 109     | range_NeighDiff_shell1_NdUnfilled       |
| 47      | var_NeighDiff_shell1_Electronegativity | 110     | mean_NeighDiff_shell1_NpValence         |
| 48      | mean_NeighDiff_shell1_MeltingT         | 111     | var_NeighDiff_shell1_NpUnfilled         |
| 49      | min_NeighDiff_shell1_Electronegativity | 112     | min_NeighDiff_shell1_AtomicWeight       |
| 50      | max_NeighDiff_shell1_NpUnfilled        | 113     | max_EffectiveCoordination               |
| 51      | range_NeighDiff_shell1_NdValence       | 114     | min_NeighDiff_shell1_Column             |
| 52      | var_NeighDiff_shell1_GSvolume_pa       | 115     | range_NeighDiff_shell1_NpUnfilled       |
| 53      | mean_EffectiveCoordination             | 116     | var_NeighDiff_shell1_NUnfilled          |
| 54      | range_NeighDiff_shell1_GSmagmom        | 117     | max_NeighDiff_shell1_NdValence          |
| 55      | max_NeighDiff_shell1_NfValence         | 118     | range_NeighDiff_shell1_Column           |
| 56      | var_MeanBondLength                     | 119     | mean_NeighDiff_shell1_NUnfilled         |

| Sr. No. | Feature Name                       | Sr. No. | Feature Name                           |
|---------|------------------------------------|---------|----------------------------------------|
| 57      | mean_NeighDiff_shell1_GSmagmom     | 120     | var_NeighDiff_shell1_MendelevNumber    |
| 58      | var_NeighDiff_shell1_NpValence     | 121     | max_NeighDiff_shell1_Electronegativity |
| 59      | range_NeighDiff_shell1_GSvolume_pa | 122     | max_NeighDiff_shell1_NsUnfilled        |
| 60      | mean_BondLengthVariation           | 123     | max_NeighDiff_shell1_CovalentRadius    |
| 61      | max_NeighDiff_shell1_NfUnfilled    | 124     | range_NeighDiff_shell1_MendelevNumber  |
| 62      | mean_NeighDiff_shell1_Column       | 125     | mean_NeighDiff_shell1_NValance         |
| 63      | var_CellVolume                     | 126     | range_NeighDiff_shell1_NUnfilled       |

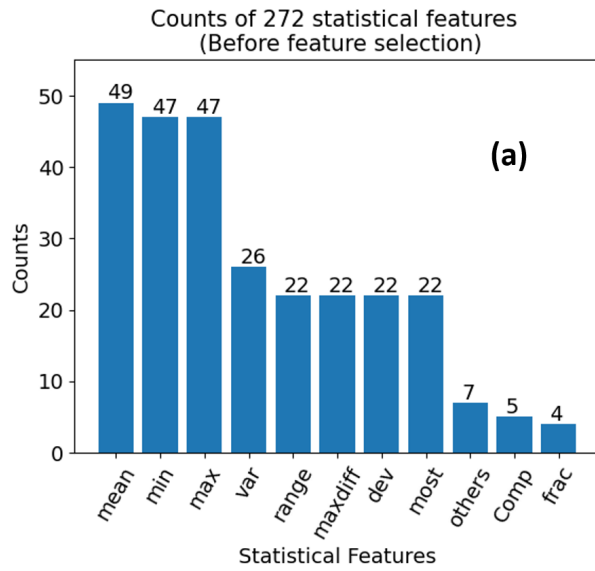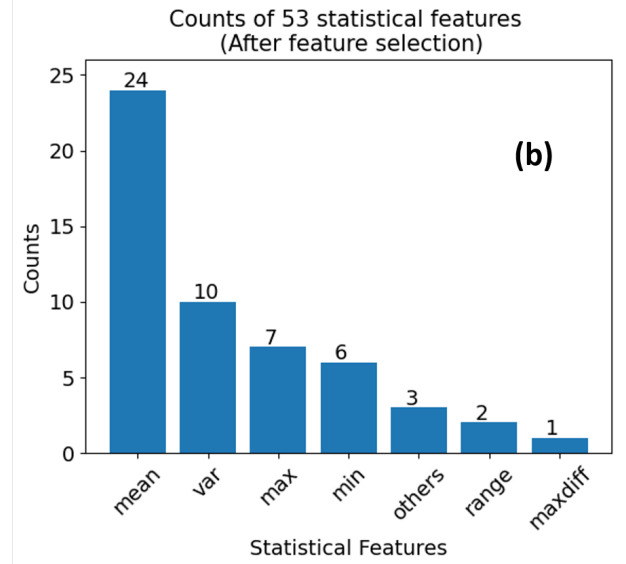

FIG. S2. Distribution of Statistical features (a) before feature selection (271 Features) (b) after feature selection (53 Features)

TABLE S6. Selected features for model training and their abbreviations used for Pearson Correlation analysis plot.

| Feature Name                           | Abbr. | Feature Name                           | Abbr. |
|----------------------------------------|-------|----------------------------------------|-------|
| Temperature                            | F1    | var_NeighDiff_shell1_GSvolume_pa       | F28   |
| mean_EffectiveCoordination             | F2    | mean_NeighDiff_shell1_GSbandgap        | F29   |
| var_EffectiveCoordination              | F3    | range_NeighDiff_shell1_GSbandgap       | F30   |
| mean_NeighDiff_shell1_Number           | F4    | mean_NeighDiff_shell1_SpaceGroupNumber | F31   |
| var_NeighDiff_shell1_Number            | F5    | var_NeighDiff_shell1_SpaceGroupNumber  | F32   |
| mean_NeighDiff_shell1_MendeleevNumber  | F6    | NComp                                  | F33   |
| var_NeighDiff_shell1_MendeleevNumber   | F7    | mean_Number                            | F34   |
| mean_NeighDiff_shell1_MeltingT         | F8    | max_MendeleevNumber                    | F35   |
| var_NeighDiff_shell1_MeltingT          | F9    | mean_MeltingT                          | F36   |
| mean_NeighDiff_shell1_CovalentRadius   | F10   | min_MeltingT                           | F37   |
| var_NeighDiff_shell1_CovalentRadius    | F11   | mean_CovalentRadius                    | F38   |
| max_NeighDiff_shell1_Electronegativity | F12   | mean_NpValence                         | F39   |
| max_NeighDiff_shell1_NsValence         | F13   | min_NpValence                          | F40   |
| mean_NeighDiff_shell1_NpValence        | F14   | mean_NdValence                         | F41   |
| mean_NeighDiff_shell1_NdValence        | F15   | max_NdValence                          | F42   |
| var_NeighDiff_shell1_NdValence         | F16   | min_NdValence                          | F43   |
| mean_NeighDiff_shell1_NfValence        | F17   | min_NfValence                          | F44   |
| var_NeighDiff_shell1_NfValence         | F18   | mean_NpUnfilled                        | F45   |
| mean_NeighDiff_shell1_NValance         | F19   | max_NpUnfilled                         | F46   |
| max_NeighDiff_shell1_NsUnfilled        | F20   | mean_NUnfilled                         | F47   |
| mean_NeighDiff_shell1_NpUnfilled       | F21   | min_NUnfilled                          | F48   |
| range_NeighDiff_shell1_NpUnfilled      | F22   | min_GSvolume_pa                        | F49   |
| mean_NeighDiff_shell1_NdUnfilled       | F23   | maxdiff_GSmagmom                       | F50   |
| mean_NeighDiff_shell1_NfUnfilled       | F24   | mean_SpaceGroupNumber                  | F51   |
| mean_NeighDiff_shell1_NUnfilled        | F25   | max_SpaceGroupNumber                   | F52   |
| var_NeighDiff_shell1_NUnfilled         | F26   | CanFormIonic                           | F53   |
| mean_NeighDiff_shell1_GSvolume_pa      | F27   |                                        |       |



### III. MACHINE LEARNING MODELS:

In this study, a variety of supervised machine learning (ML) models were employed to train and validate the temperature-dependent lattice thermal conductivity ( $\kappa_L$ ) of 150 compounds using their corresponding feature vectors as input. All ML models were implemented using the scikit-learn[23] python library and trained using default hyperparameters. The regression models evaluated in this work include:

(1) **Decision Tree:** A non-parametric, tree-based algorithm that recursively splits the dataset based on feature values, resulting in a hierarchical decision structure. Although simple and interpretable, it is often susceptible to overfitting but serves as a foundational model for many ensemble methods[24].

(2) **Random Forest:** An ensemble learning method that builds multiple decision trees on randomly sampled subsets of the data and features, and averages their outputs to reduce variance and improve generalization [25].

(3) **Extreme Gradient Boosting (XGBoost):** An optimized implementation of gradient boosting that incorporates regularization, pruning, and parallelization for efficient, accurate, and scalable learning[26].

(4) **Gradient Boosting Regressor:** A sequential ensemble model where each new tree corrects the prediction errors of the previous trees by optimizing a loss function. It is known for strong predictive performance but typically requires careful tuning of hyperparameters[27].

(5) **AdaBoost Regressor (with Decision Trees):** Adaptive Boosting combines multiple weak learners (decision trees) by reweighting the training instances, focusing more on those that were previously misclassified, to iteratively improve prediction accuracy[28].

(6) **Bagging Regressor (with Decision Trees):** Bootstrap aggregation (bagging) involves training multiple decision trees on different random subsets of the training data and aggregating their outputs, reducing model variance and improving robustness[29].

(7) **Extra Trees Regressor:** A variant of the Random Forest model, Extra Trees introduces additional randomness in selecting the features and threshold at each split, often resulting in a more generalized and diverse model[30].

TABLE S7. Global average feature importance scores of Extra Trees Regressor model.

| Sr.No. | Feature Name                           | Feature Importance Score |
|--------|----------------------------------------|--------------------------|
| 1      | Temperature                            | $1.35 \times 10^{-1}$    |
| 2      | mean_NpUnfilled                        | $1.31 \times 10^{-1}$    |
| 3      | min_NUnfilled                          | $1.06 \times 10^{-1}$    |
| 4      | min_GSvolume_pa                        | $7.03 \times 10^{-2}$    |
| 5      | mean_EffectiveCoordination             | $6.55 \times 10^{-2}$    |
| 6      | mean_CovalentRadius                    | $6.28 \times 10^{-2}$    |
| 7      | mean_NUnfilled                         | $3.16 \times 10^{-2}$    |
| 8      | mean_NeighDiff_shell1_MeltingT         | $3.01 \times 10^{-2}$    |
| 9      | mean_Number                            | $2.32 \times 10^{-2}$    |
| 10     | range_NeighDiff_shell1_NpUnfilled      | $1.89 \times 10^{-2}$    |
| 11     | mean_MeltingT                          | $1.87 \times 10^{-2}$    |
| 12     | max_NpUnfilled                         | $1.71 \times 10^{-2}$    |
| 13     | NComp                                  | $1.53 \times 10^{-2}$    |
| 14     | mean_NpValence                         | $1.53 \times 10^{-2}$    |
| 15     | mean_NeighDiff_shell1_GSvolume_pa      | $1.51 \times 10^{-2}$    |
| 16     | var_NeighDiff_shell1_NUnfilled         | $1.44 \times 10^{-2}$    |
| 17     | min_NdValence                          | $1.38 \times 10^{-2}$    |
| 18     | var_EffectiveCoordination              | $1.32 \times 10^{-2}$    |
| 19     | max_NeighDiff_shell1_Electronegativity | $1.25 \times 10^{-2}$    |
| 20     | var_NeighDiff_shell1_MendeleevNumber   | $1.22 \times 10^{-2}$    |
| 21     | min_NpValence                          | $1.18 \times 10^{-2}$    |
| 22     | mean_NeighDiff_shell1_NfValence        | $1.13 \times 10^{-2}$    |
| 23     | var_NeighDiff_shell1_GSvolume_pa       | $1.13 \times 10^{-2}$    |
| 24     | var_NeighDiff_shell1_CovalentRadius    | $1.12 \times 10^{-2}$    |
| 25     | max_MendeleevNumber                    | $1.07 \times 10^{-2}$    |
| 26     | mean_NeighDiff_shell1_NpUnfilled       | $9.11 \times 10^{-3}$    |
| 27     | mean_NeighDiff_shell1_MendeleevNumber  | $8.37 \times 10^{-3}$    |

| Sr.No. | Feature Name                           | Feature Importance Score |
|--------|----------------------------------------|--------------------------|
| 28     | var_NeighDiff_shell1_MeltingT          | $7.36 \times 10^{-3}$    |
| 29     | mean_NdValence                         | $7.33 \times 10^{-3}$    |
| 30     | max_NeighDiff_shell1_NsValence         | $6.54 \times 10^{-3}$    |
| 31     | mean_NeighDiff_shell1_CovalentRadius   | $6.43 \times 10^{-3}$    |
| 32     | mean_NeighDiff_shell1_NdUnfilled       | $5.98 \times 10^{-3}$    |
| 33     | mean_NeighDiff_shell1_NpValence        | $5.94 \times 10^{-3}$    |
| 34     | var_NeighDiff_shell1_Number            | $5.15 \times 10^{-3}$    |
| 35     | range_NeighDiff_shell1_GSbandgap       | $4.68 \times 10^{-3}$    |
| 36     | CanFormIonic                           | $4.64 \times 10^{-3}$    |
| 37     | mean_NeighDiff_shell1_NUnfilled        | $4.49 \times 10^{-3}$    |
| 38     | max_SpaceGroupNumber                   | $4.46 \times 10^{-3}$    |
| 39     | var_NeighDiff_shell1_SpaceGroupNumber  | $4.45 \times 10^{-3}$    |
| 40     | mean_NeighDiff_shell1_Number           | $4.37 \times 10^{-3}$    |
| 41     | var_NeighDiff_shell1_NdValence         | $4.18 \times 10^{-3}$    |
| 42     | mean_NeighDiff_shell1_NdValence        | $4.05 \times 10^{-3}$    |
| 43     | min_MeltingT                           | $4.01 \times 10^{-3}$    |
| 44     | mean_SpaceGroupNumber                  | $3.80 \times 10^{-3}$    |
| 45     | mean_NeighDiff_shell1_NValance         | $3.58 \times 10^{-3}$    |
| 46     | mean_NeighDiff_shell1_GSbandgap        | $3.45 \times 10^{-3}$    |
| 47     | mean_NeighDiff_shell1_SpaceGroupNumber | $3.41 \times 10^{-3}$    |
| 48     | max_NeighDiff_shell1_NsUnfilled        | $2.03 \times 10^{-3}$    |
| 49     | max_NdValence                          | $1.68 \times 10^{-3}$    |
| 50     | var_NeighDiff_shell1_NfValence         | $1.59 \times 10^{-3}$    |
| 51     | mean_NeighDiff_shell1_NfUnfilled       | $9.51 \times 10^{-4}$    |
| 52     | maxdiff_GSmagmom                       | $9.43 \times 10^{-4}$    |
| 53     | min_NfValence                          | $3.36 \times 10^{-5}$    |

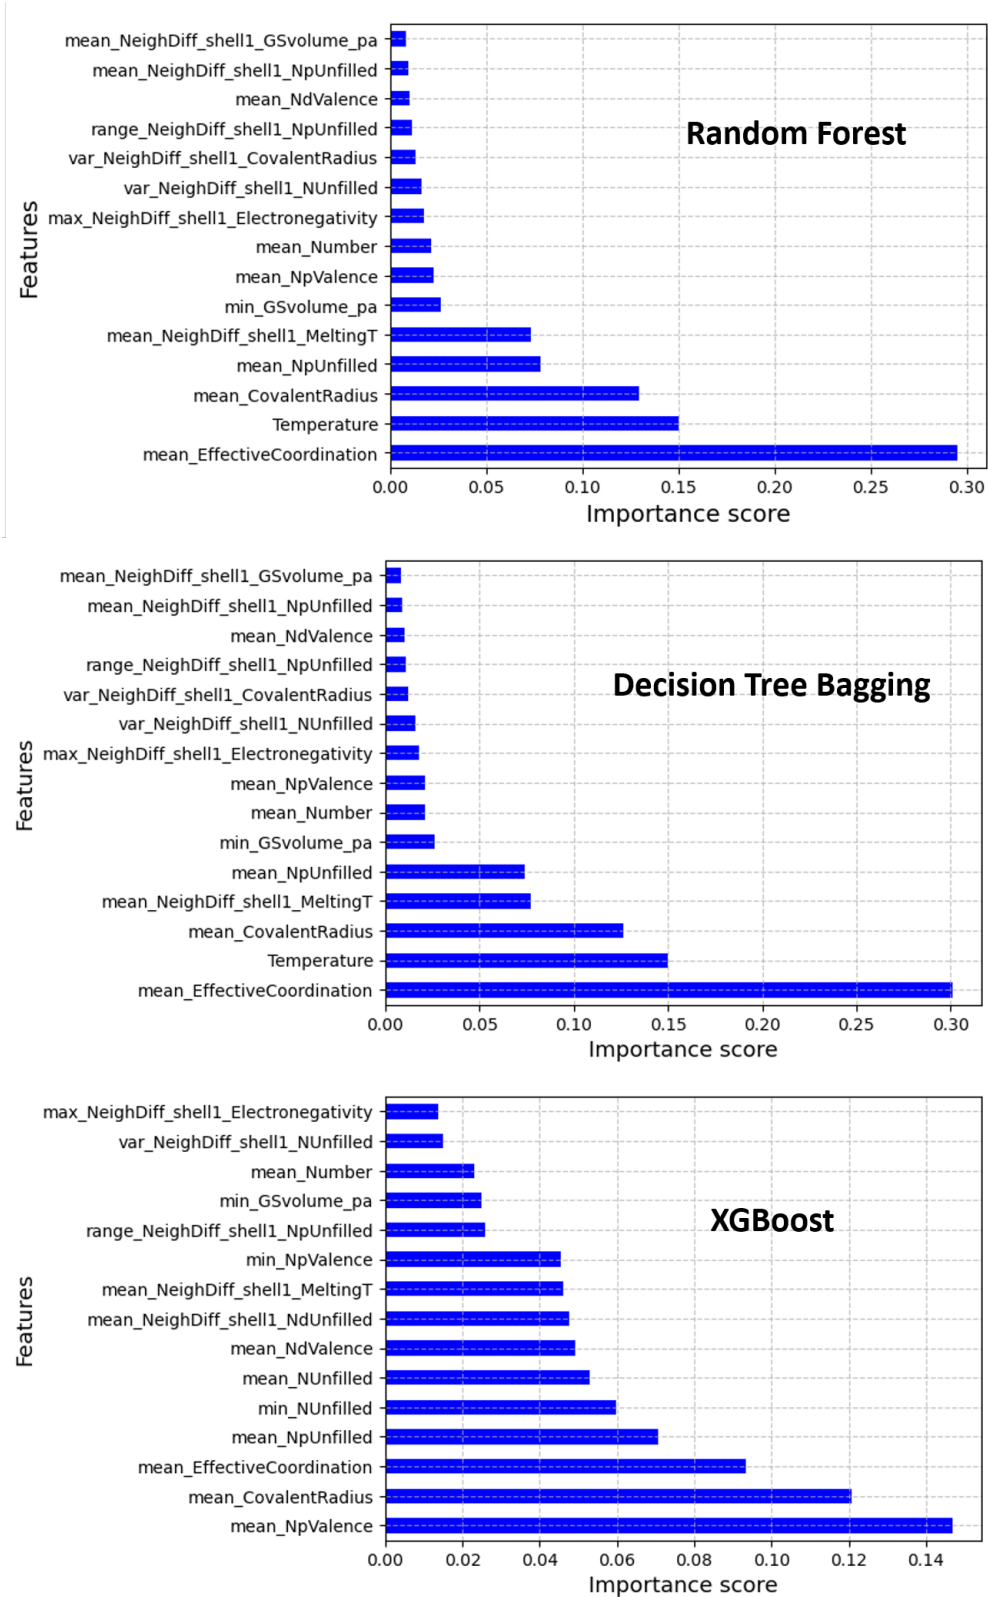

FIG. S3. Feature importance scores of Random Forest, Decision Tree Bagging and XGBoost models.

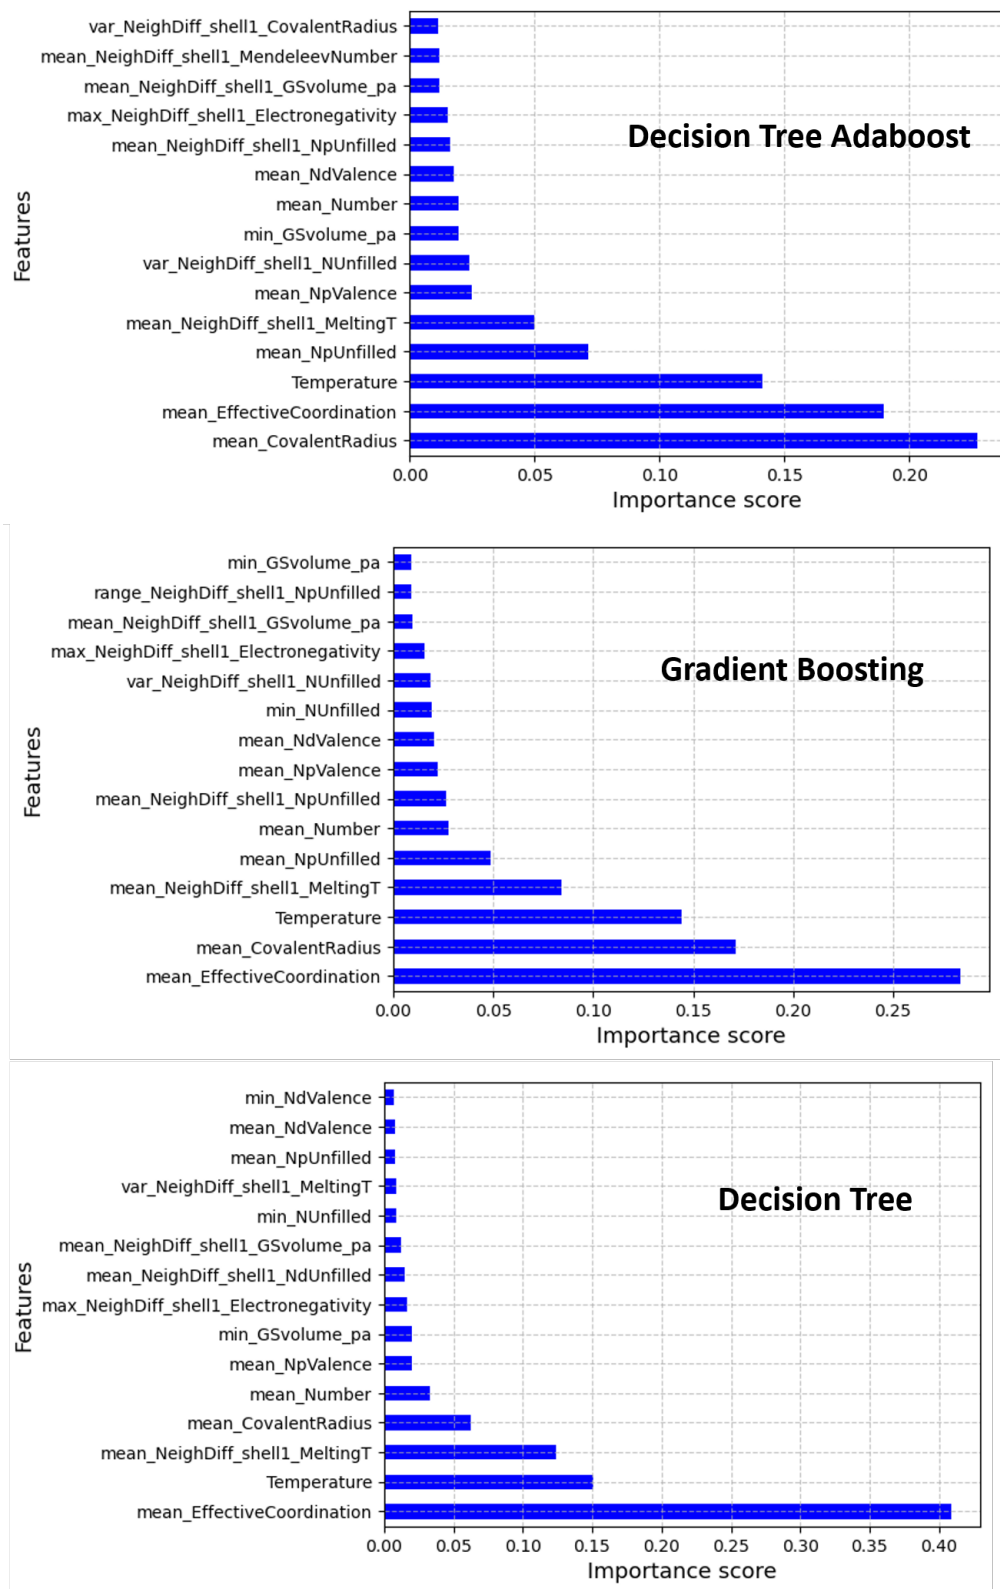

FIG. S4. Feature importance scores of Decision Tree Adaboost, Gradient Boosting and Decision Tree models.

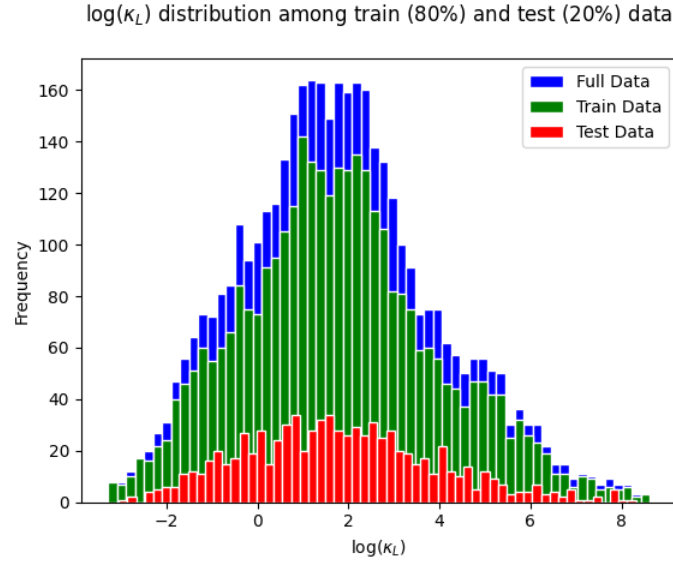

FIG. S5. Train-Test data distribution of  $\log(\kappa_L)$  for model training and testing.

- 
- [1] Rinkle Juneja, George Yumnam, Swanti Satsangi, and Abhishek K. Singh. Coupling the high-throughput property map to machine learning for predicting lattice thermal conductivity. *Chemistry of Materials*, 31(14):5145–5151, 2019.
  - [2] Fan Mo, Tingting Zhang, Suiting Ning, Ning Qi, and Zhiquan Chen. Thermoelectric performance of  $\text{Ag}_2\text{GeX}_3$  ( $X = \text{S}, \text{Se}, \text{Te}$ ) with intrinsically low lattice thermal conductivity: A first principles study. *Physica B: Condensed Matter*, 690:416217, 2024.
  - [3] Prakash Govindaraj, Kowsalya Murugan, and Kathirvel Venugopal. Role of lattice thermal conductivity in thermoelectric properties of chalcopyrite-type antimonides  $\text{XSiSb}_2$  ( $X = \text{Mg}, \text{Be}$ ): A dft insight. *Materials Chemistry and Physics*, 295:127190, 2023.
  - [4] Yucong He and Jian Zhou. First-principles study on the ultralow lattice thermal conductivity of  $\text{BiSeI}$ . *Physica B: Condensed Matter*, 646:414278, 2022.
  - [5] Jian Zhang, Haochun Zhang, Jie Xiong, Shuai Chen, and Gang Zhang. Theoretical insights into the lattice thermal conductivity and thermal expansion of  $\text{CoNiFe}$  medium-entropy alloys. *Mater. Adv.*, 5:3998–4005, 2024.
  - [6] Enamul Haque. First-principles predictions of low lattice thermal conductivity and high thermoelectric performance of  $\text{AZnSb}$  ( $A = \text{Rb}, \text{Cs}$ ). *RSC Adv.*, 11(25):15486–15496, 2021. Publisher: The Royal Society of Chemistry.
  - [7] Vineet Kumar Sharma, V. Kanchana, Mayanak K. Gupta, and Ranjan Mittal. Topological phonons and low lattice thermal conductivity of  $\text{Li}_2\text{CaX}$  ( $X = \text{Sn}$  and  $\text{Pb}$ ) type heusler compounds. *Materials Today Communications*, 35:106289, 2023.
  - [8] Cong Wang, Y. B. Chen, Shu-Hua Yao, and Jian Zhou. Low lattice thermal conductivity and high thermoelectric figure of merit in  $\text{Na}_2\text{MgSn}$ . *Phys. Rev. B*, 99:024310, Jan 2019.
  - [9] Xue-Liang Zhu, Peng-Fei Liu, Yi-Yuan Wu, Ping Zhang, Guofeng Xie, and Bao-Tian Wang. Significant enhancement of the thermoelectric properties of  $\text{CaP}_3$  through reducing the dimensionality. *Mater. Adv.*, 1(9):3322–3332, 2020. Publisher: RSC.
  - [10] Luc Andrea, Gilles Hug, and Laurent Chaput. Ab initio phonon properties of half-heusler  $\text{NiTiSn}$ ,  $\text{NiZrSn}$  and  $\text{NiHfSn}$ . *Journal of Physics: Condensed Matter*, 27(42):425401, oct 2015.
  - [11] Junhong Wei, Yongliang Guo, and Guangtao Wang. Exploring structural, mechanical, and thermoelectric properties of half-heusler compounds  $\text{RhBiX}$  ( $X = \text{Ti}, \text{Zr}, \text{Hf}$ ): A first-principles

- investigation. *RSC Adv.*, 13:11513–11524, 2023.
- [12] Hao-Jen You, Bo-Ying Su, Yi-Ting Chiang, Tse-Hsiao Li, Hsu-Shen Chu, and Hsin Lin. First-principles study on the thermoelectric properties of  $\text{Sr}_2\text{Si}$  and  $\text{Sr}_2\text{Ge}$ . *Materials Today Physics*, 32:101015, 2023.
- [13] Elkana Rugut, Daniel Joubert, and Glenn Jones. First principle studies on lattice thermal conductivity and thermoelectric properties of  $\text{ScCu}(\text{S,Se,Te})_2$ . *Materials Today Communications*, 26:101905, 2021.
- [14] Dingfeng Yang, Shuling Chen, Hongzheng Pu, Mingyu Pi, and Yuanyuan Li. Large difference of lattice thermal conductivity between thermoelectric compounds  $\text{Cu}_3\text{VSe}_4$  and  $\text{Tl}_3\text{VSe}_4$ : Elasticity, anharmonicity and chemical bonding from first-principles calculation. *Materials Today Communications*, 37:107505, 2023.
- [15] LDDI–Laboratory, Faculty of Science and Technology, University Ahmed Draia of Adrar,01000, Algeria, M. Guenfoud, M. Hamouda, and LDDI–Laboratory, Faculty of Science and Technology, University Ahmed Draia of Adrar,01000, Algeria. Thermal conductivity and lattice dynamics of thermoelectric oxychalcogenide  $\text{BiCuTeO}$ . *Chalcogenide Letters*, 20(10):697–708, November 2023.
- [16] Appala Naidu Gandhi and Udo Schwingenschlögl. Thermoelectric properties of the  $\text{XCoSb}$  (X: Ti,Zr,Hf) half-Heusler alloys. *physica status solidi (b)*, 254(11):1700419, 2017.
- [17] Xin Luo, Tian Zhang, Cui-E Hu, Yan Cheng, and Hua-Yun Geng. First-principles studies on the structural, electronic and thermal transport characteristics of half-Heusler compounds  $\text{LiXN}$  (X=Mg, Zn). *Solid State Communications*, 366-367:115156, 2023.
- [18] Sukhwinder Singh. Assessing the thermoelectric properties of  $\text{Sr}_2\text{HfTe}_6$  half-Heusler compound. *Computational Condensed Matter*, 13:120–126, 2017.
- [19] Jaspal Singh, Kulwinder Kaur, Ishtihadah Islam, Jan Mohammad Mir, Megha Goyal, Tavneet Kaur, S.S. Verma, Atif Mossad Ali, and Shakeel Ahmad Khandy. Electronic structure, phonon stability, mechanical and high-temperature thermoelectric properties of Li-based quaternary Heusler alloys. *Current Applied Physics*, 50:161–167, 2023.
- [20] F. Parvin, M.A. Hossain, I. Ahmed, K. Akter, and A.K.M.A. Islam. First-principles calculations to investigate mechanical, optoelectronic and thermoelectric properties of half-Heusler p-type semiconductor  $\text{BaAgP}$ . *Results in Physics*, 23:104068, 2021.
- [21] Magpie- <https://bitbucket.org/wolverton/magpie/src/master/>.



- [22] Logan Ward, Ankit Agrawal, Alok Choudhary, and Christopher Wolverton. A general-purpose machine learning framework for predicting properties of inorganic materials. *npj Computational Materials*, 2:16028, 2016.
- [23] Fabian Pedregosa, Gaël Varoquaux, Alexandre Gramfort, Vincent Michel, Bertrand Thirion, Olivier Grisel, Mathieu Blondel, Peter Prettenhofer, Ron Weiss, Vincent Dubourg, Jake Vanderplas, Alexandre Passos, David Cournapeau, Matthieu Brucher, Matthieu Perrot, and Édouard Duchesnay. Scikit-learn: Machine learning in python. *J. Mach. Learn. Res.*, 12(null):2825–2830, November 2011.
- [24] Leo Breiman, Jerome H Friedman, Richard A Olshen, and Charles J Stone. *Classification and Regression Trees*. Wadsworth International Group, 1984.
- [25] Leo Breiman. Random forests. *Machine Learning*, 45(1):5–32, 2001.
- [26] Tianqi Chen and Carlos Guestrin. XGBoost: A scalable tree boosting system. In *Proceedings of the ACM SIGKDD International Conference on Knowledge Discovery and Data Mining (KDD)*, pages 785–794, 2016.
- [27] Jerome H Friedman. Greedy function approximation: A gradient boosting machine. *Annals of Statistics*, 29(5):1189–1232, 2001.
- [28] Yoav Freund and Robert E Schapire. A decision-theoretic generalization of on-line learning and an application to boosting. In *European Conference on Computational Learning Theory*, pages 23–37. Springer, 1995.
- [29] Leo Breiman. Bagging predictors. *Machine Learning*, 24(2):123–140, 1996.
- [30] Pierre Geurts, Damien Ernst, and Louis Wehenkel. Extremely randomized trees. *Machine Learning*, 63(1):3–42, 2006.
